# Supplementary material for: Adversarial Contrastive Learning for Evidence-aware Fake News Detection with Graph Neural Networks
Source: arXiv:2210.05498 source file (2022-10-11)
Supplement: Supplementary file 1 [file appendix.tex]

\appendices
\section{Proof of the First Zonklar Equation}
Appendix one text goes here.

% you can choose not to have a title for an appendix
% if you want by leaving the argument blank
\section{}
Appendix two text goes here.
